# Supplementary material for: Learning Large Scale Ordinary Differential Equation Systems
Source: arXiv:1710.09308 source file (2017-10-26)
Supplement: Supplementary file 1 [file supp_mat_v1.pdf]

# SUPPLEMENTARY MATERIAL: LEARNING LARGE SCALE ORDINARY DIFFERENTIAL EQUATION SYSTEMS

FREDERIK VISSING MIKKELSEN AND NIELS RICHARD HANSEN

## 1. Additional Figures

Below we present the remaining figures from the simulation studies in Section 6.

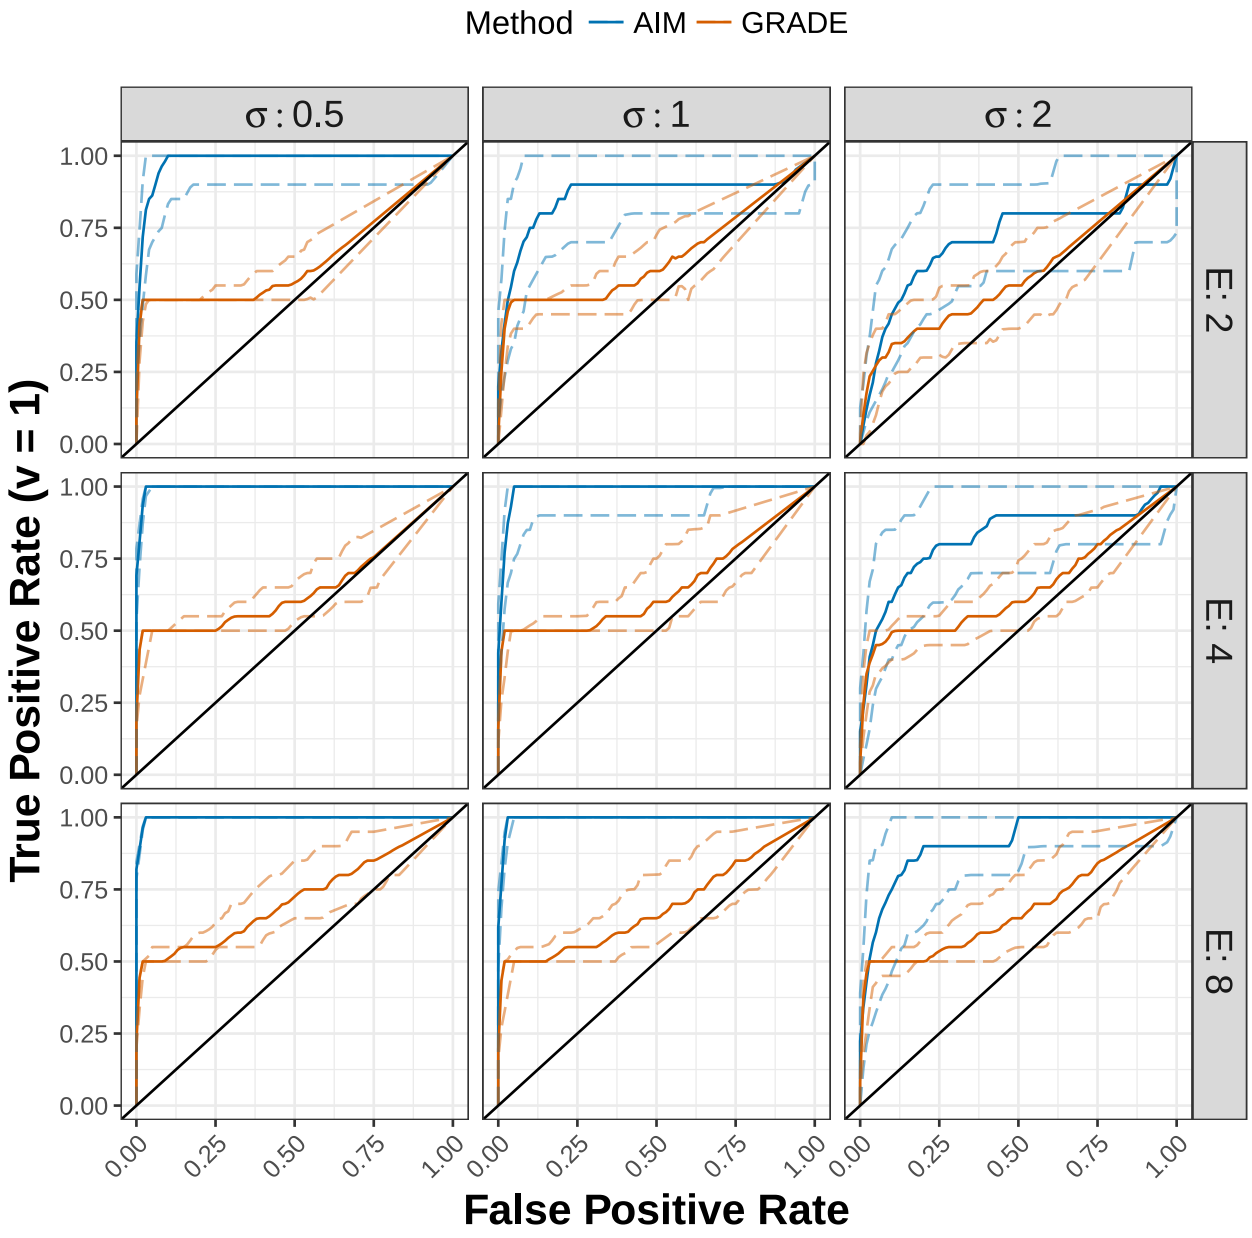
Method
AIM
GRADE
σ : 0.5
σ : 1
σ : 2
E: 2
E: 4
E: 8
True Positive Rate (v = 1)
1.00
0.75
0.50
0.25
0.00
0.00
0.25
0.50
0.75
1.00
False Positive Rate

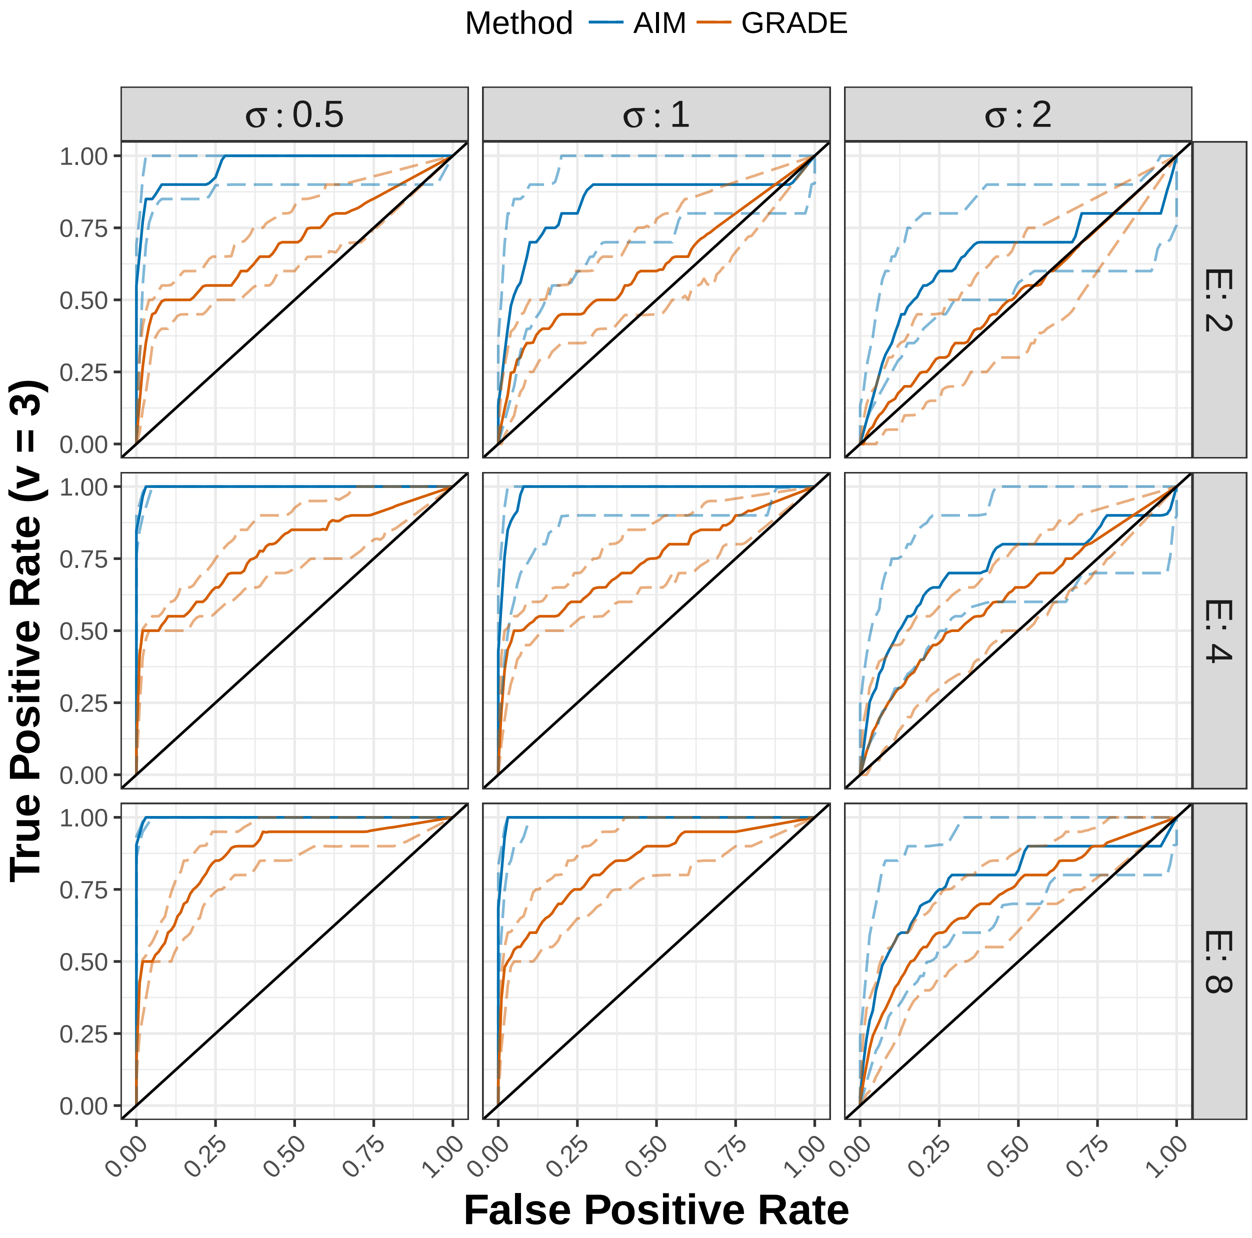

Method AIM GRADE
σ : 0.5
σ : 1
σ : 2
E: 2
E: 4
E: 8
True Positive Rate (v = 3)
False Positive Rate
0.00
0.25
0.50
0.75
1.00

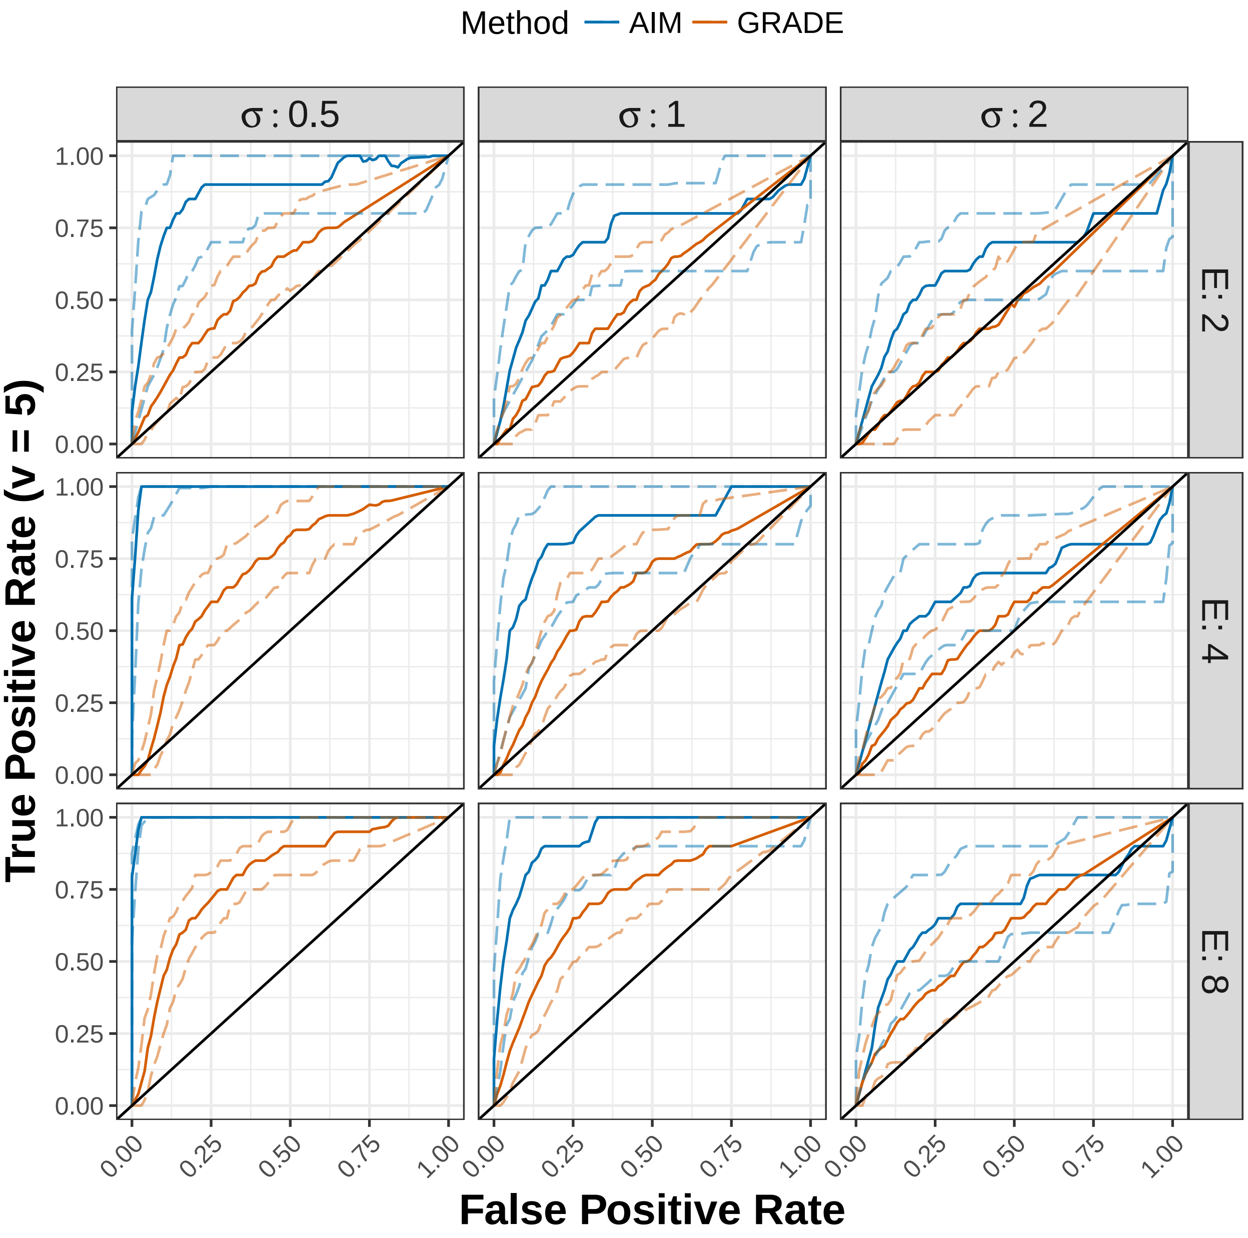

Method
AIM
GRADE
σ : 0.5
σ : 1
σ : 2
E: 2
E: 4
E: 8
True Positive Rate (v = 5)
False Positive Rate
0.00
0.25
0.50
0.75
1.00

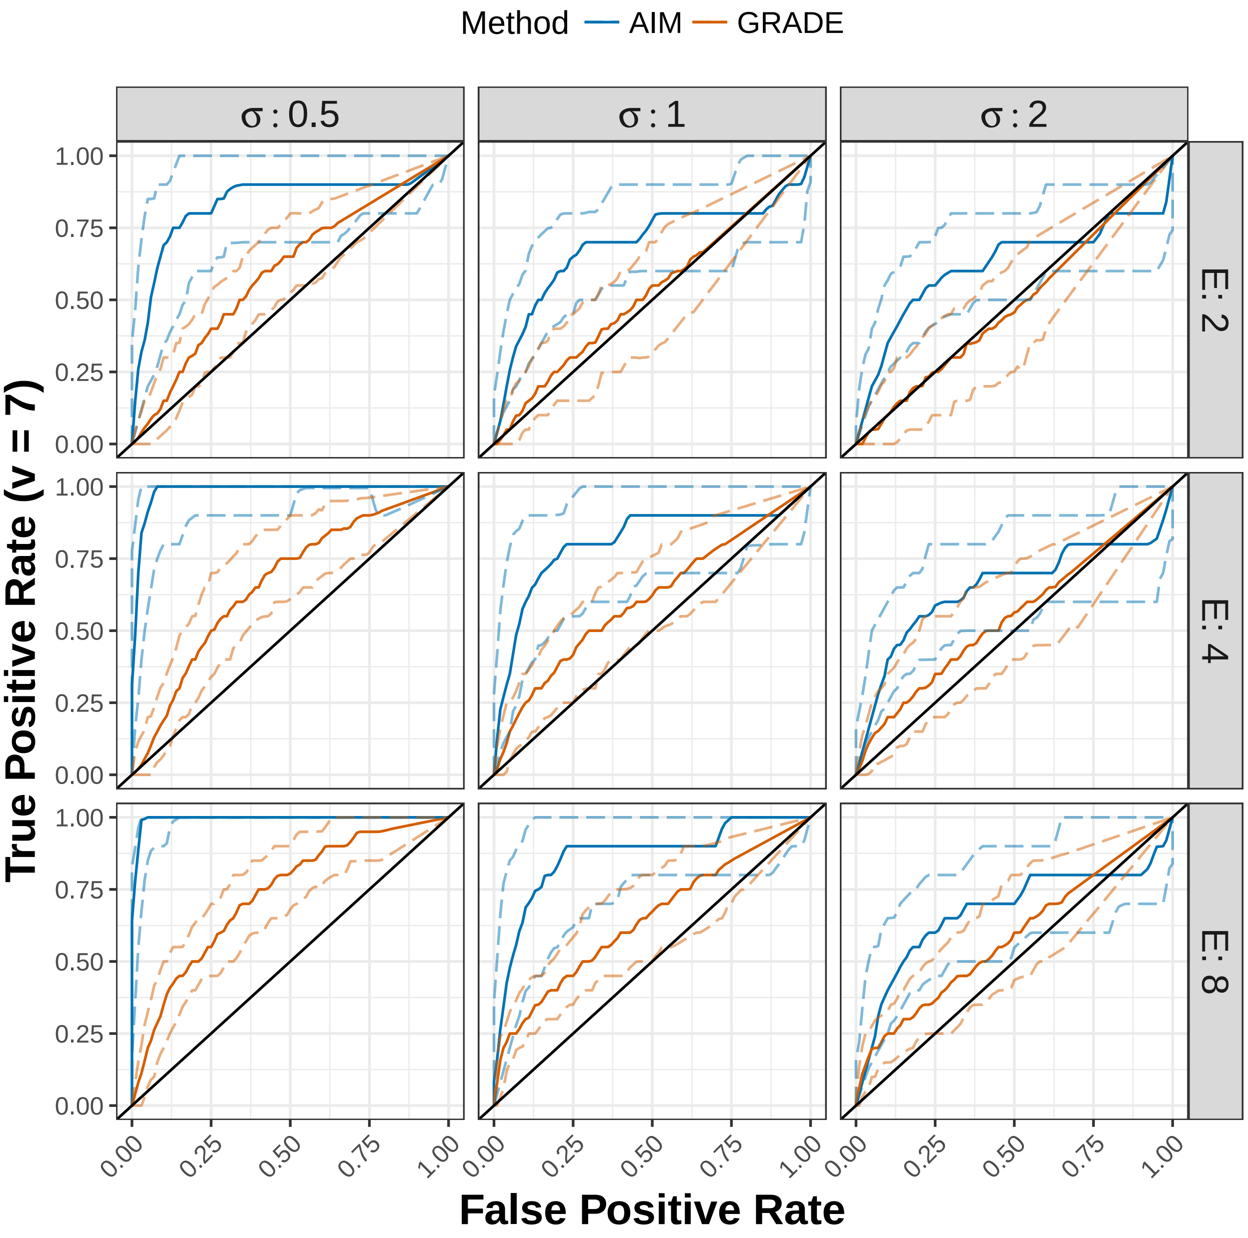

Method AIM GRADE
σ : 0.5
σ : 1
σ : 2
E: 2
E: 4
E: 8
1.00
0.75
0.50
0.25
0.00
0.00 0.25 0.50 0.75 1.00
True Positive Rate (v = 7)
False Positive Rate

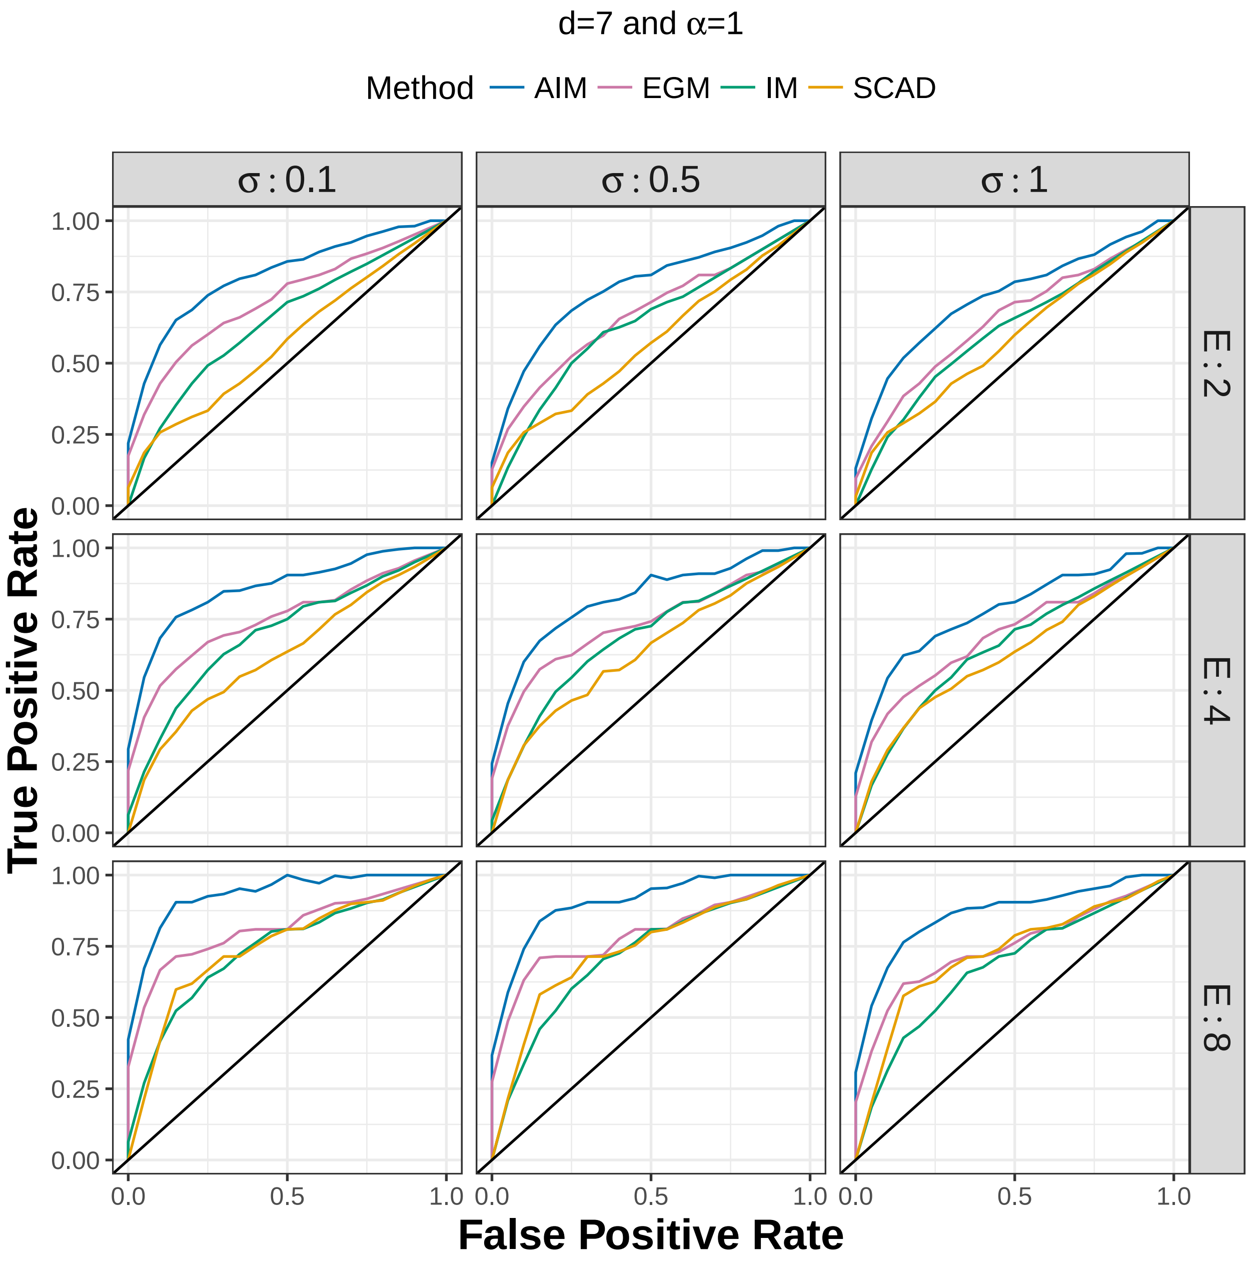
d=7 and α=1
Method AIM EGM IM SCAD
σ : 0.1
σ : 0.5
σ : 1
E : 2
E : 4
E : 8
True Positive Rate
False Positive Rate
0.00
0.25
0.50
0.75
1.00
0.0
0.5
1.0

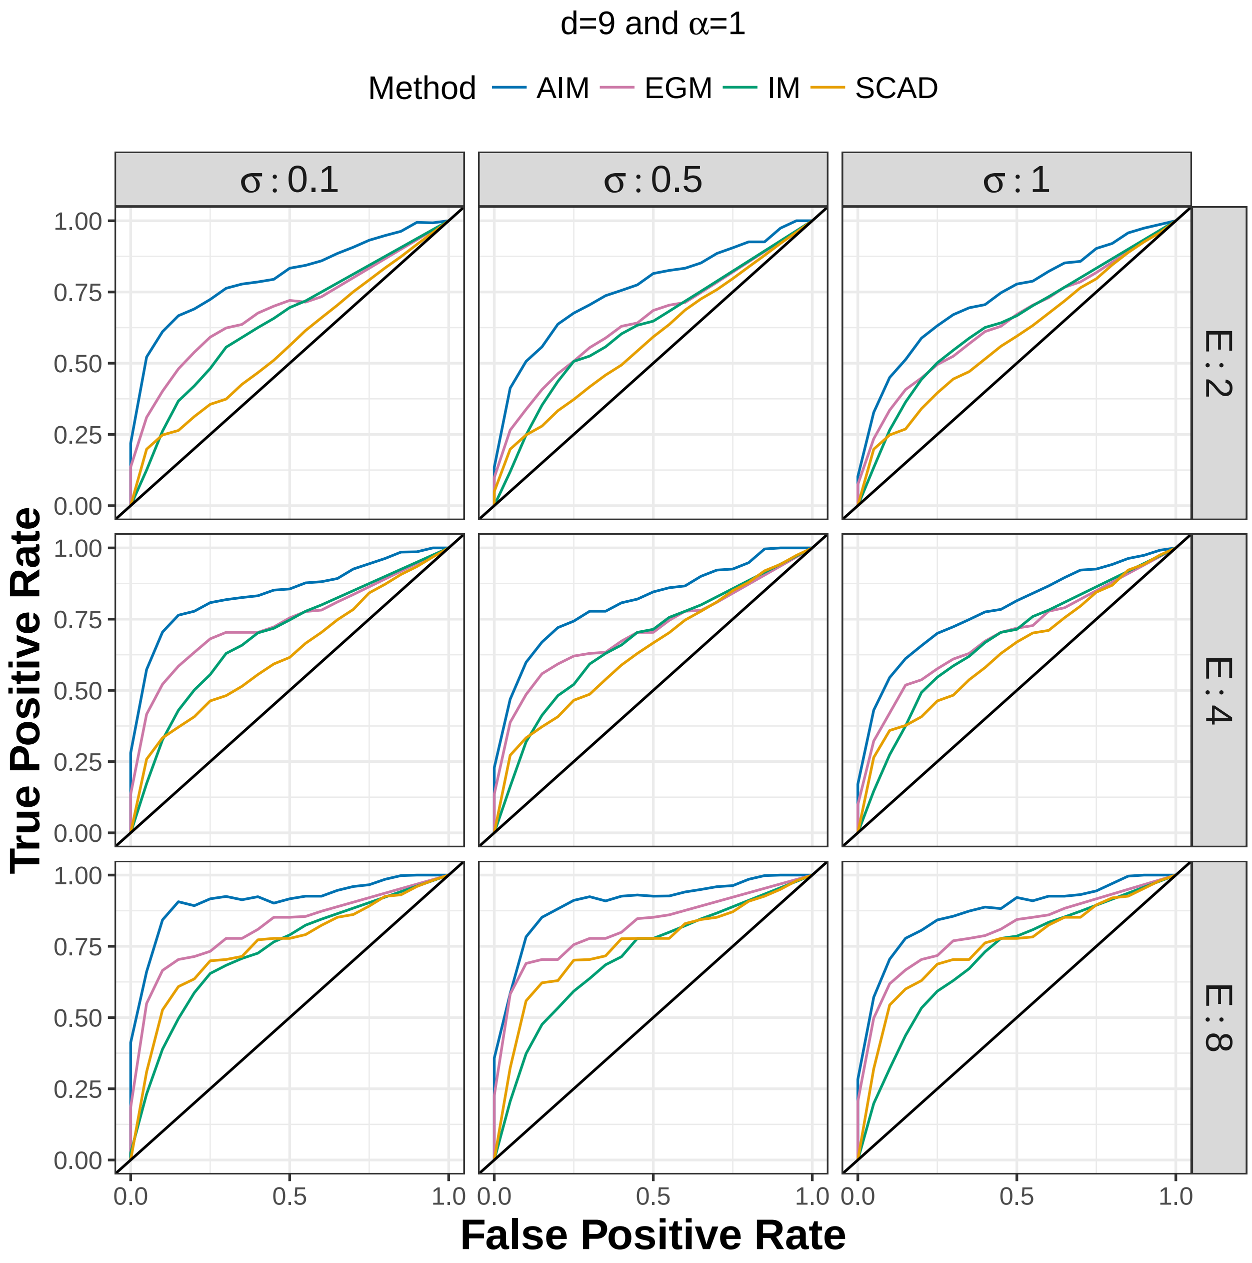

d=9 and α=1
Method AIM EGM IM SCAD
σ : 0.1
σ : 0.5
σ : 1
E : 2
E : 4
E : 8
True Positive Rate
False Positive Rate
1.00
0.75
0.50
0.25
0.00
0.0
0.5
1.0

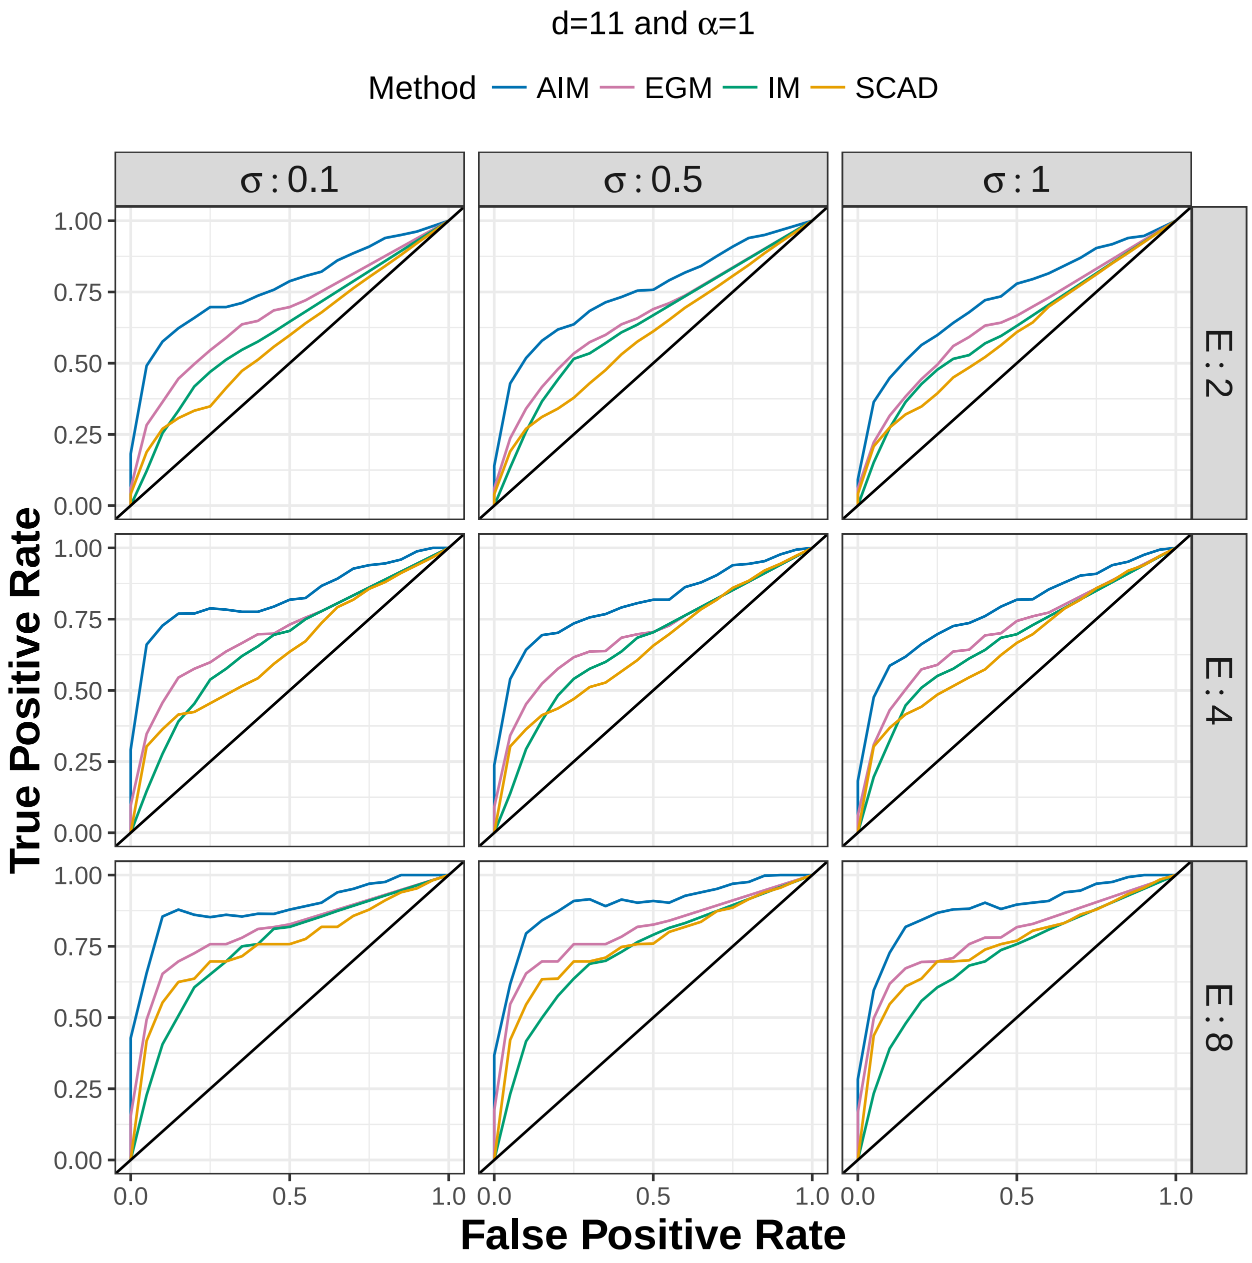

d=11 and α=1
Method AIM EGM IM SCAD
σ : 0.1
σ : 0.5
σ : 1
E : 2
E : 4
E : 8
True Positive Rate
False Positive Rate
0.00
0.25
0.50
0.75
1.00
0.0
0.5
1.0

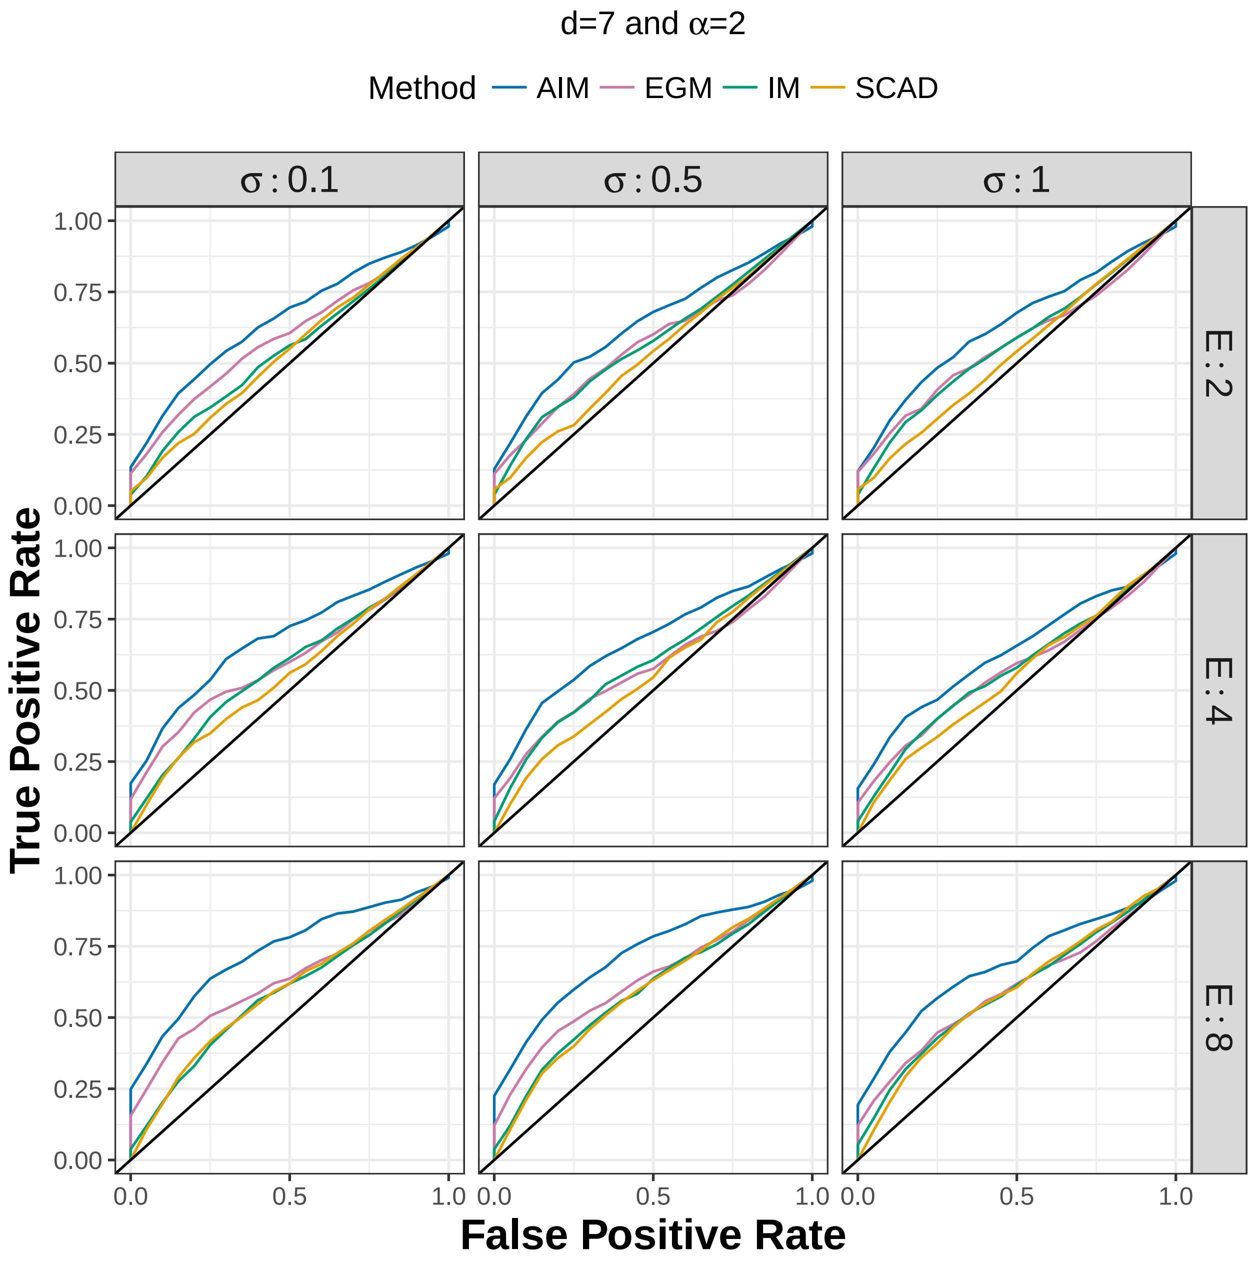

d=7 and α=2
Method
AIM
EGM
IM
SCAD
σ : 0.1
σ : 0.5
σ : 1
E : 2
E : 4
E : 8
1.00
0.75
0.50
0.25
0.00
0.0
0.5
1.0
True Positive Rate
False Positive Rate

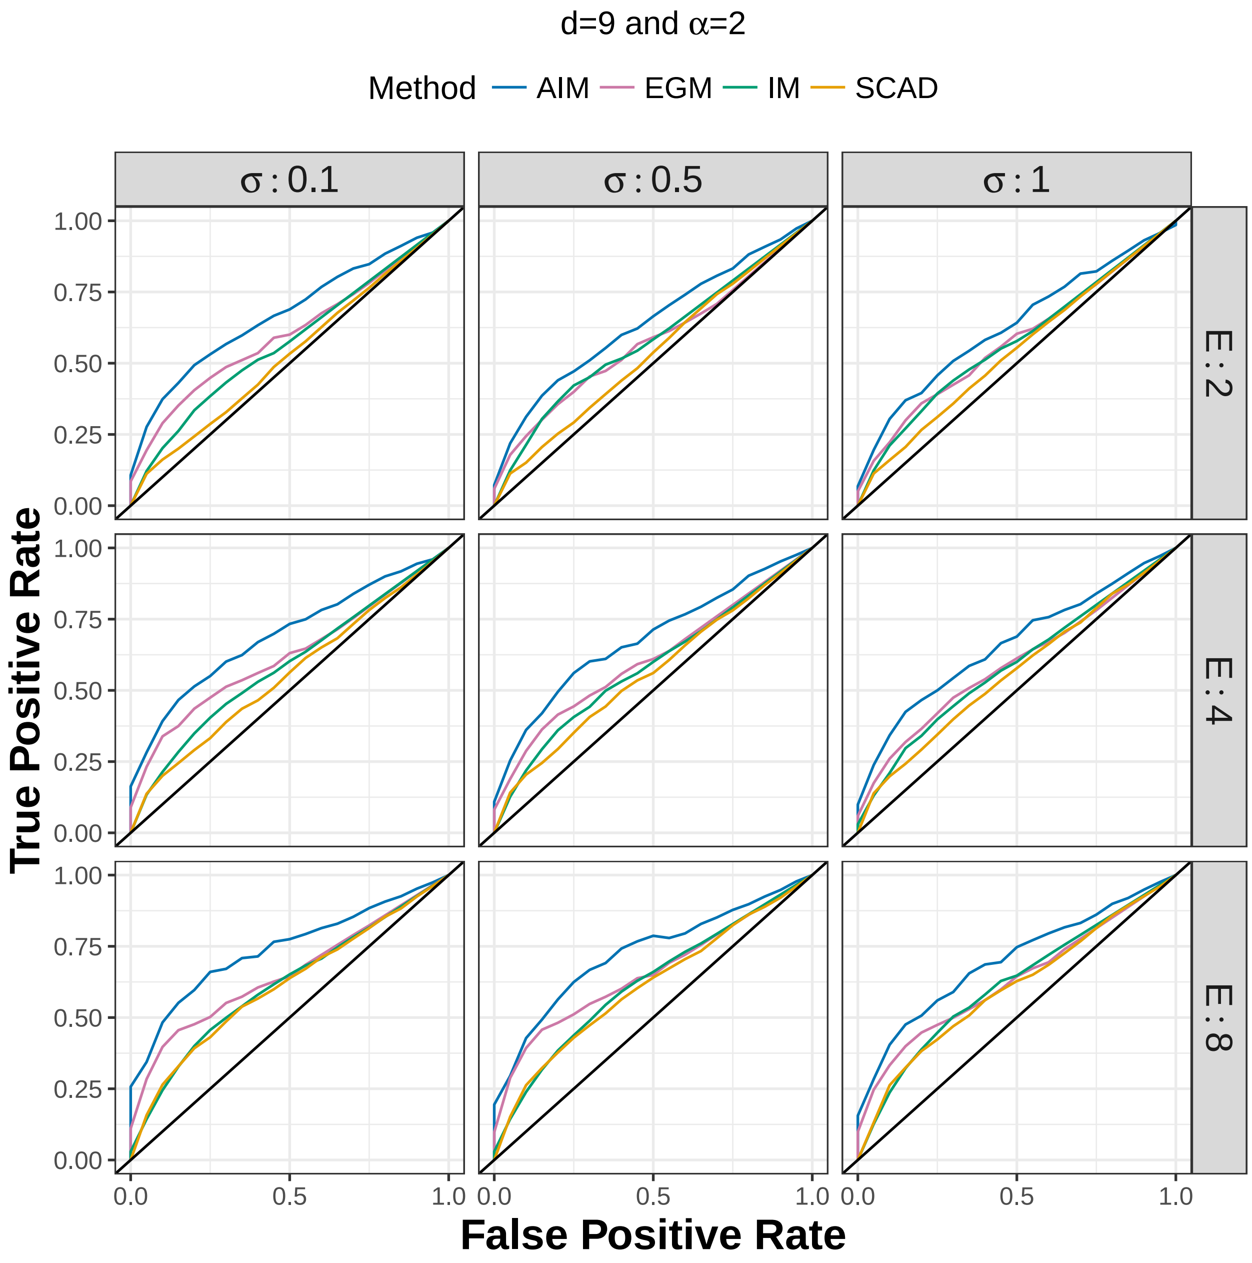

d=9 and α=2
Method AIM EGM IM SCAD
σ : 0.1
σ : 0.5
σ : 1
E : 2
E : 4
E : 8
True Positive Rate
False Positive Rate
1.00
0.75
0.50
0.25
0.00
0.0
0.5
1.0

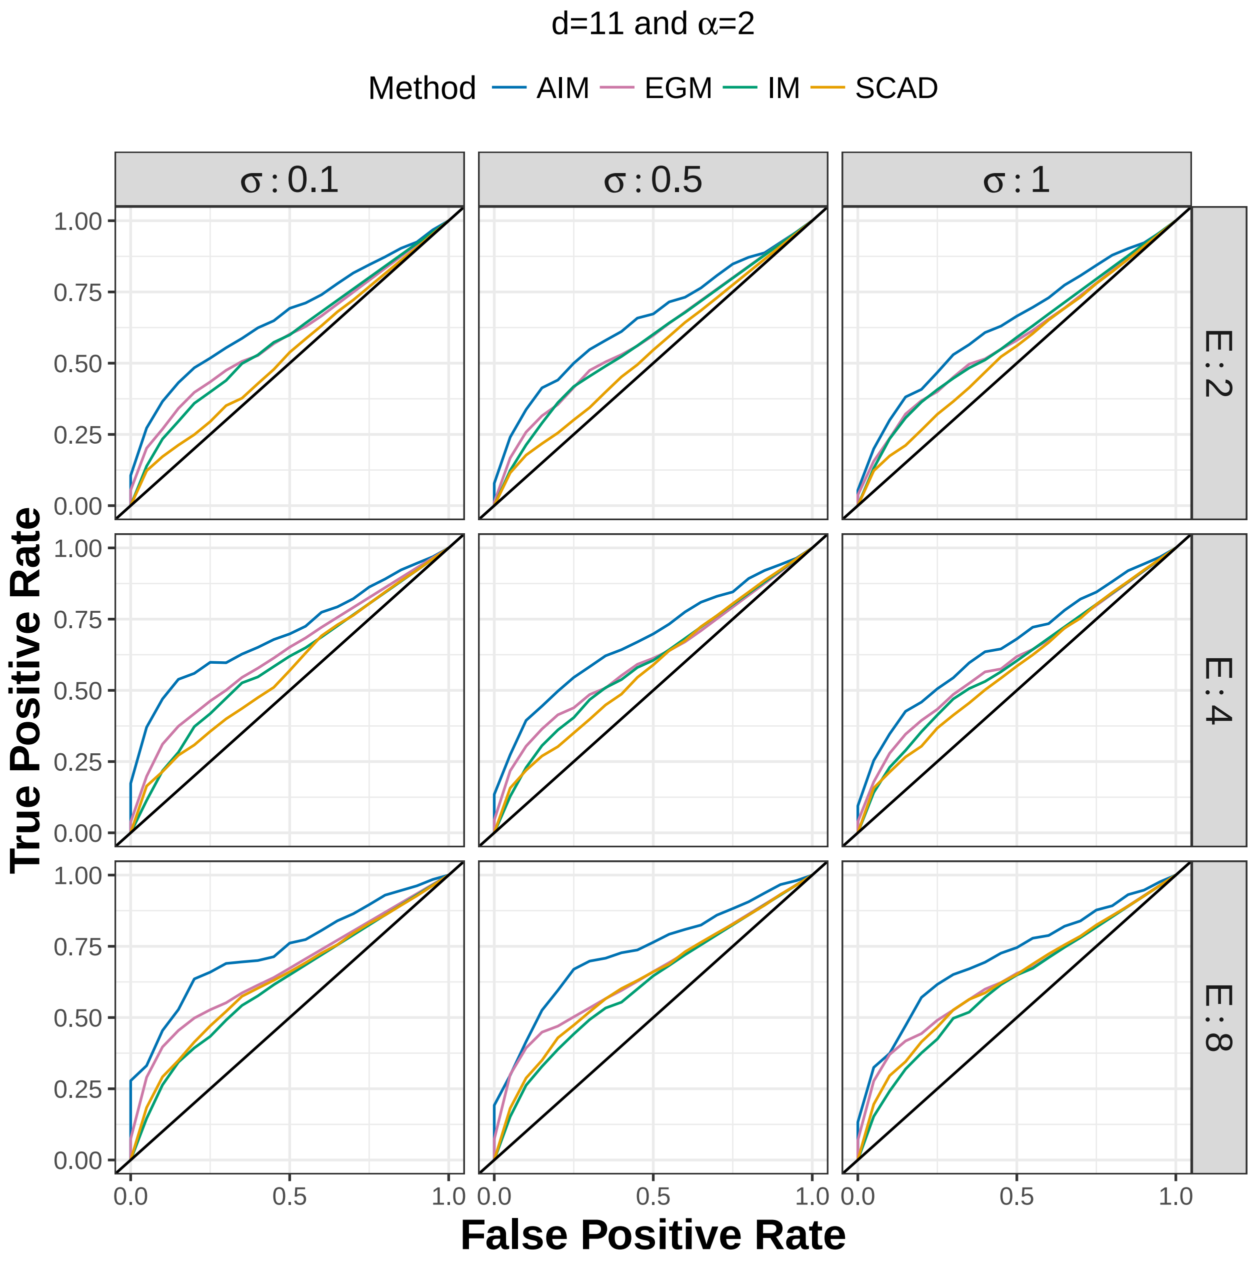
d=11 and α=2
Method
AIM
EGM
IM
SCAD
σ : 0.1
σ : 0.5
σ : 1
E : 2
E : 4
E : 8
True Positive Rate
False Positive Rate
0.00
0.25
0.50
0.75
1.00
0.0
0.5
1.0

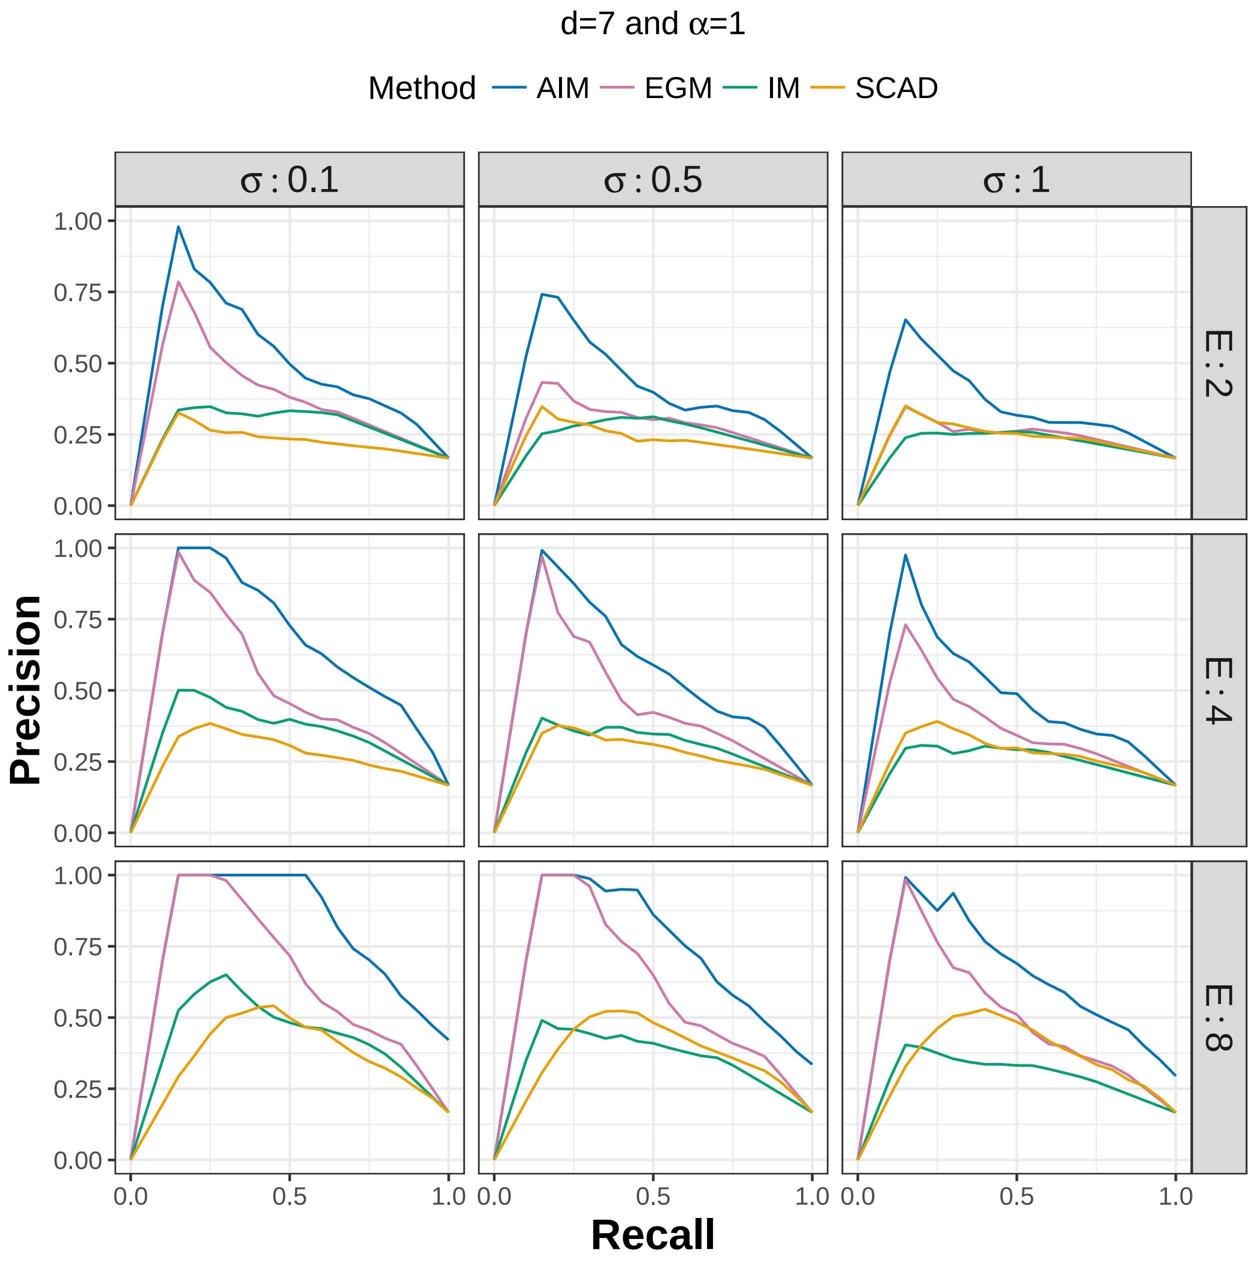
d=7 and α=1
Method
AIM
EGM
IM
SCAD
σ : 0.1
σ : 0.5
σ : 1
E : 2
E : 4
E : 8
Precision
Recall
0.00
0.25
0.50
0.75
1.00
0.0
0.5
1.0

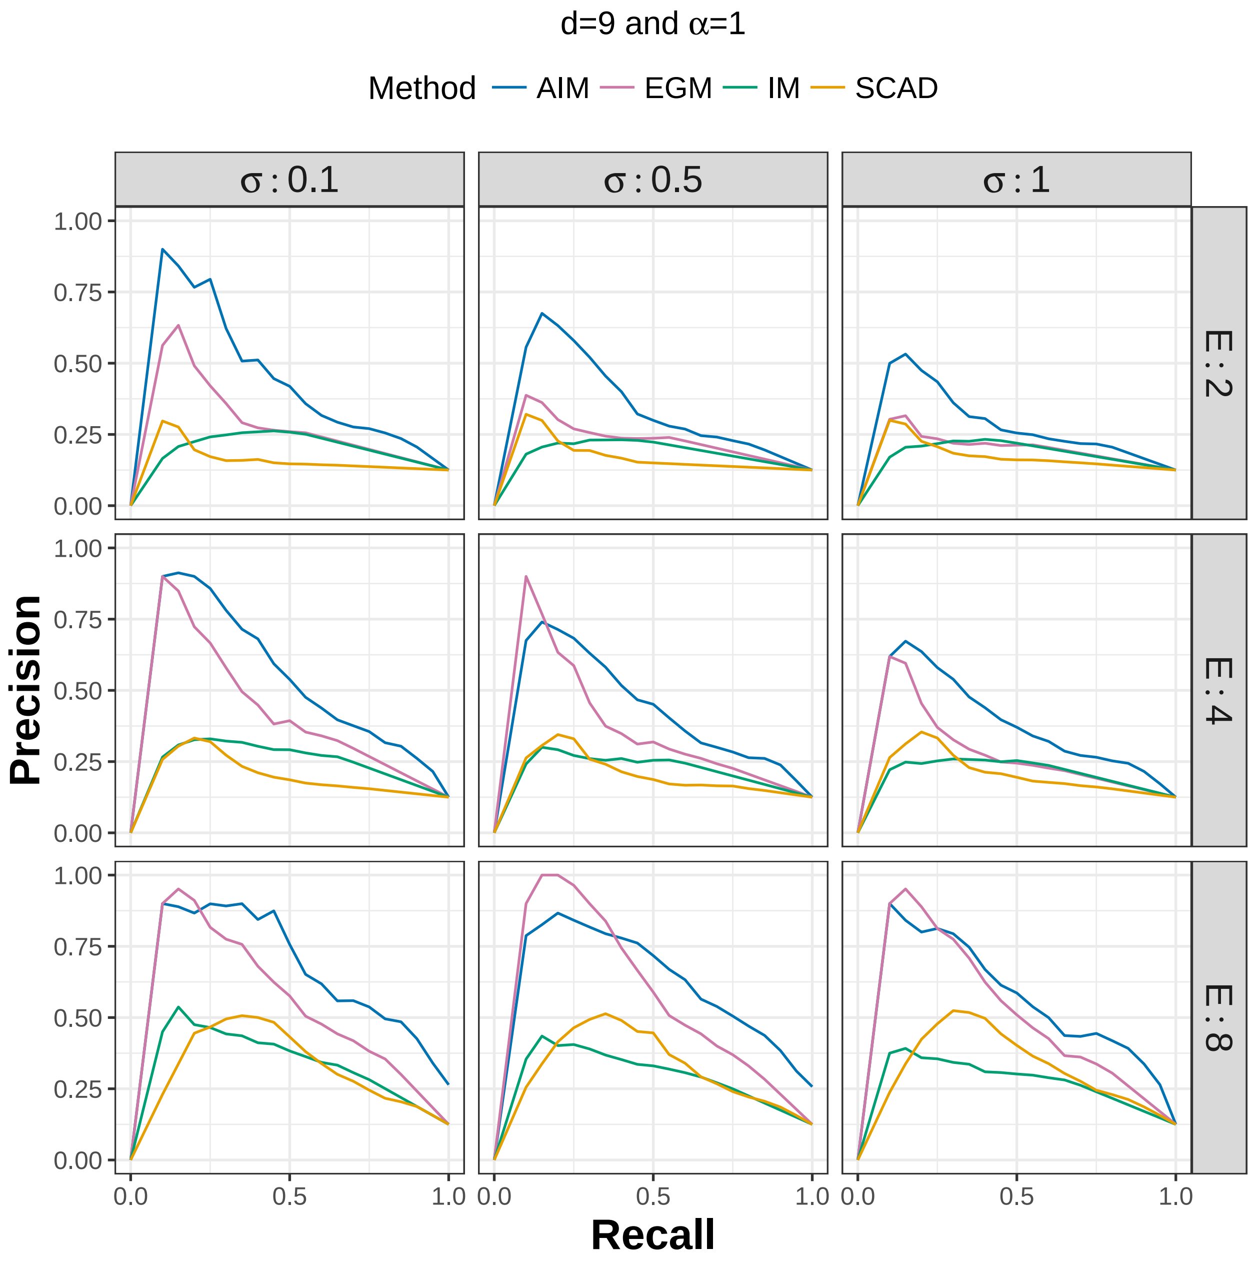
d=9 and α=1
Method AIM EGM IM SCAD
σ : 0.1
σ : 0.5
σ : 1
E : 2
E : 4
E : 8
Precision
Recall
1.00
0.75
0.50
0.25
0.00
0.0
0.5
1.0

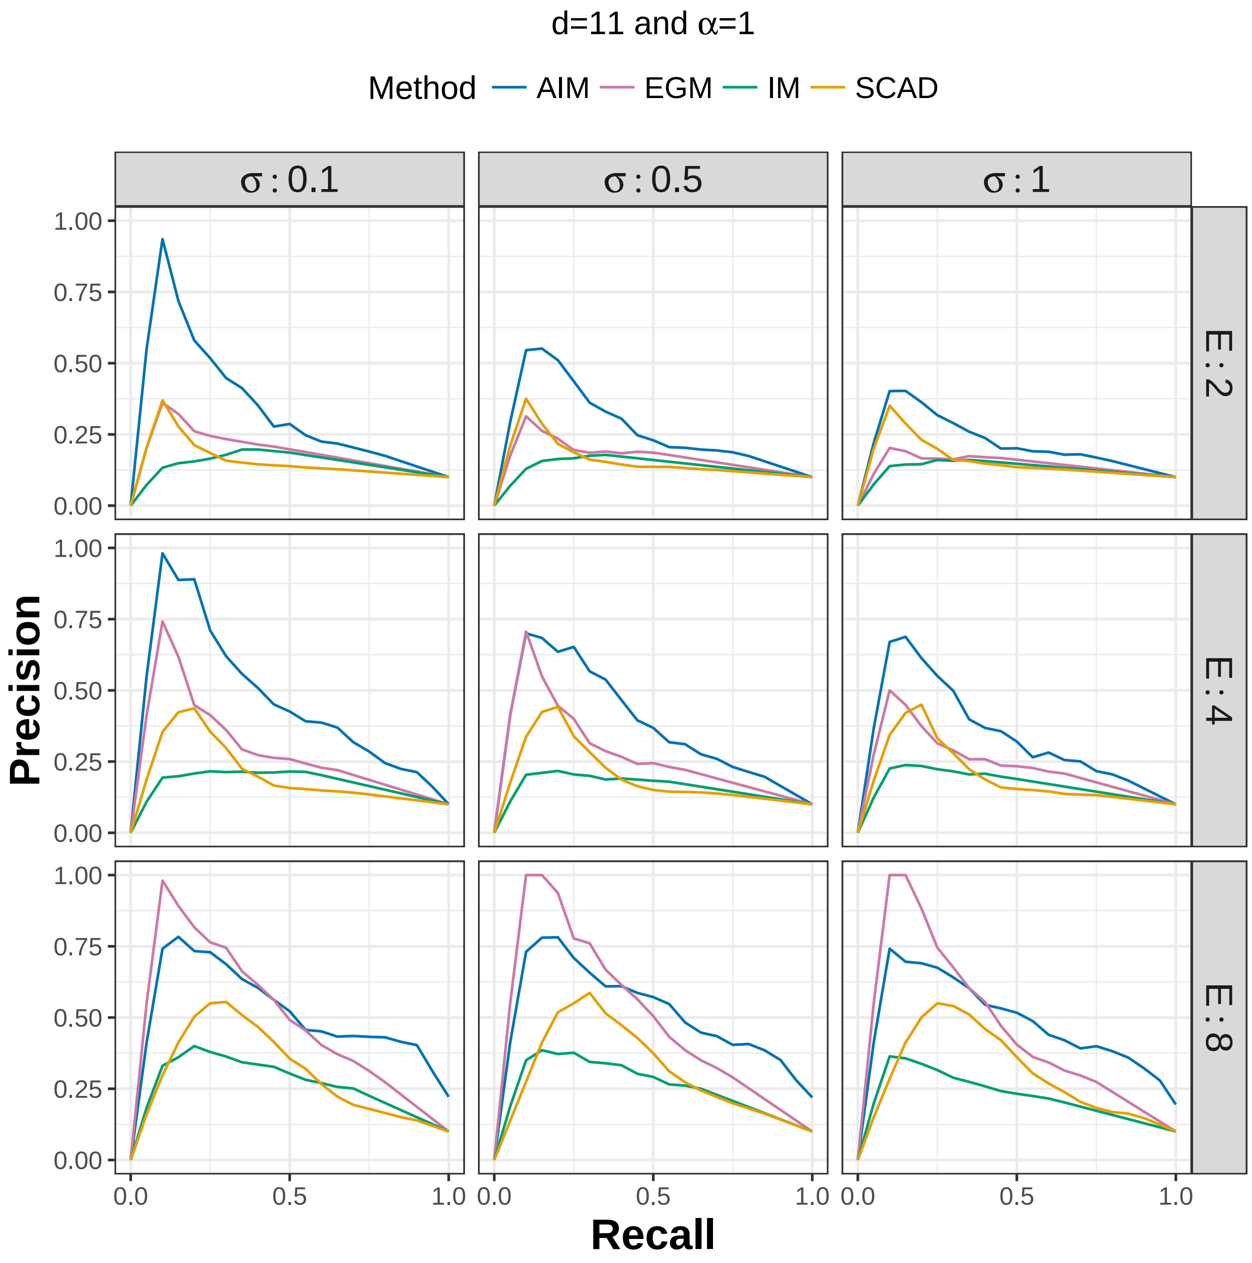
d=11 and α=1
Method AIM EGM IM SCAD
σ : 0.1
σ : 0.5
σ : 1
E : 2
E : 4
E : 8
Precision
Recall
1.00
0.75
0.50
0.25
0.00
0.0
0.5
1.0

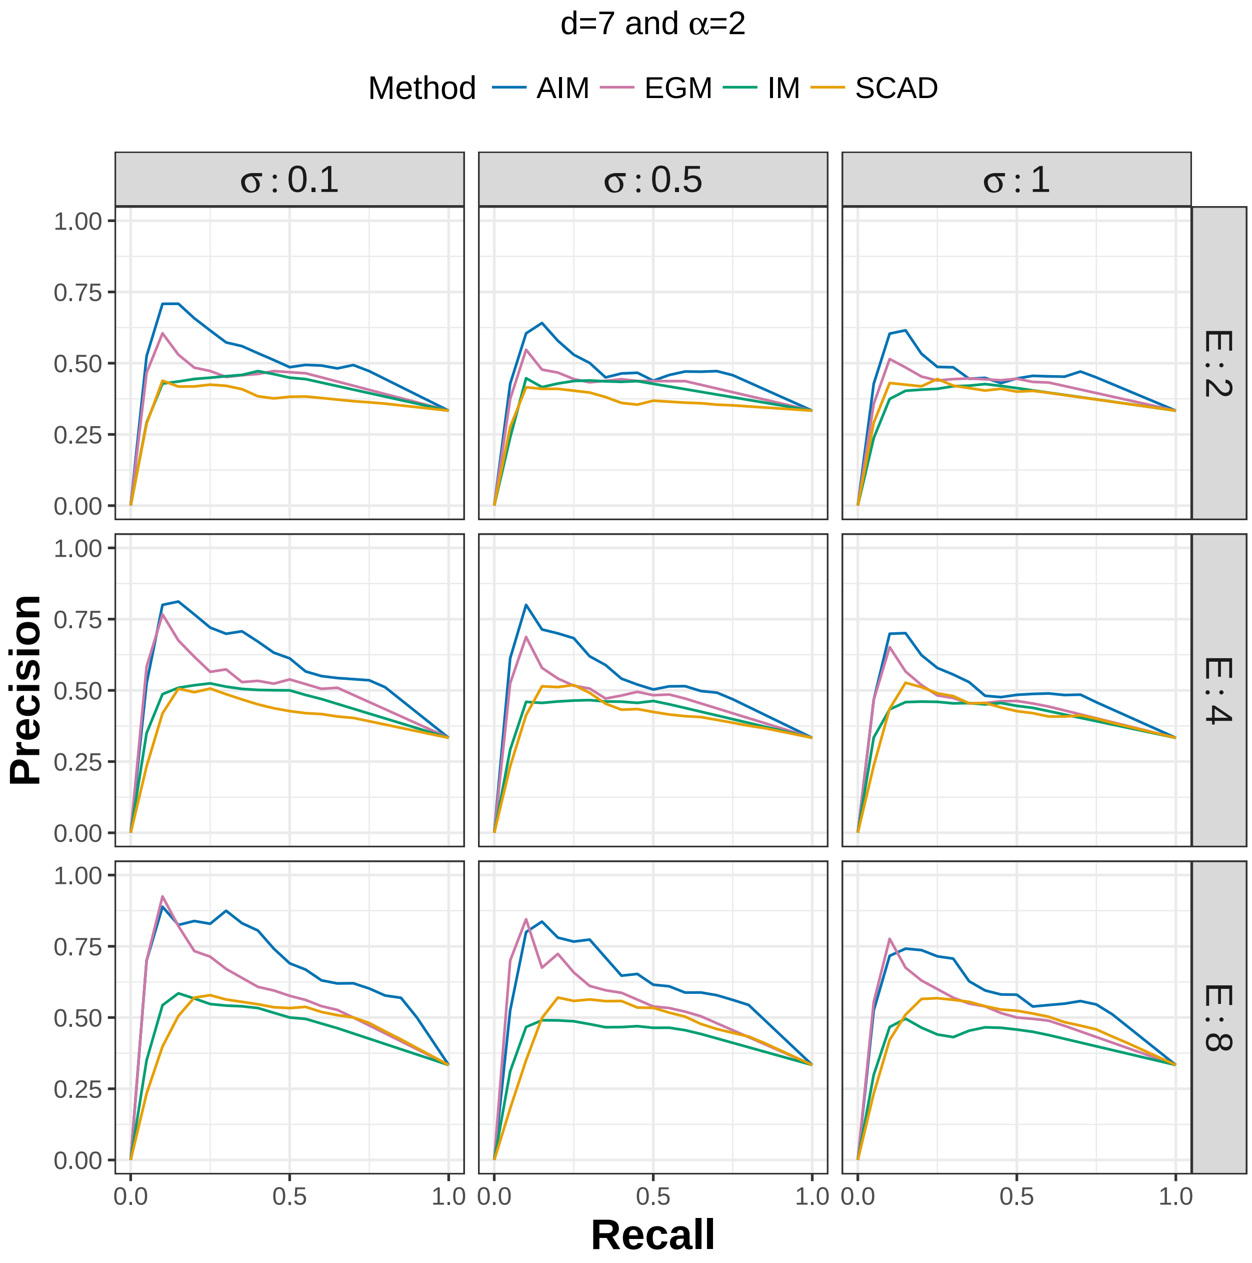
d=7 and α=2
Method
AIM
EGM
IM
SCAD
σ : 0.1
σ : 0.5
σ : 1
E : 2
E : 4
E : 8
Precision
Recall
1.00
0.75
0.50
0.25
0.00
0.0
0.5
1.0

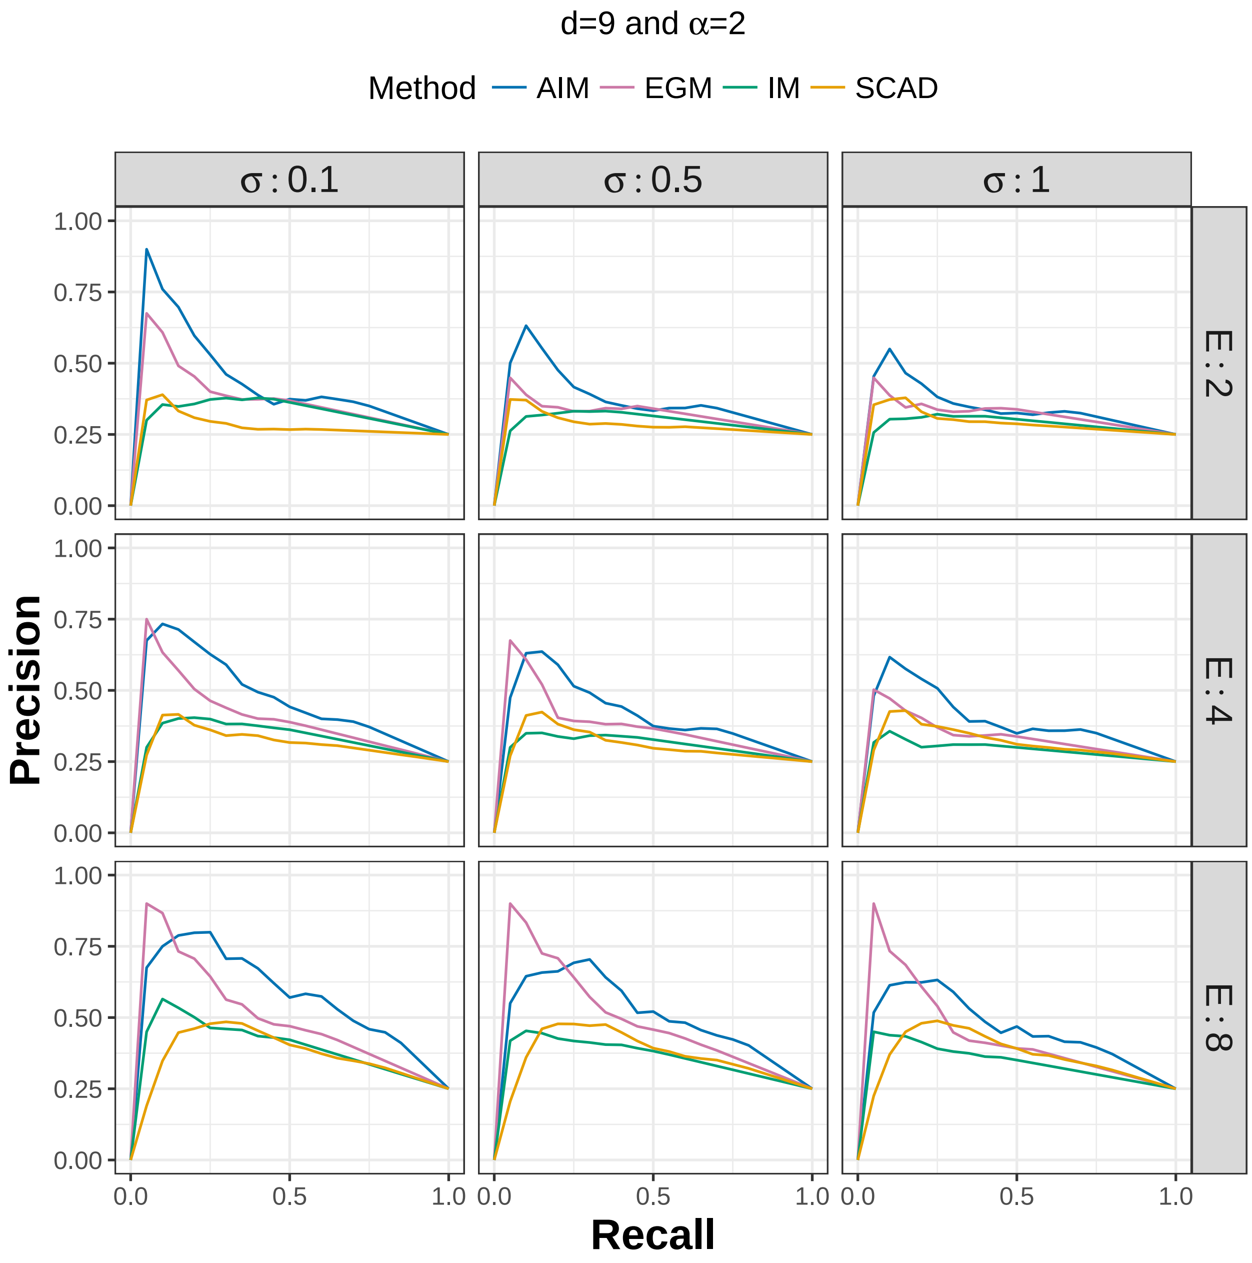
d=9 and α=2
Method
AIM
EGM
IM
SCAD
σ : 0.1
σ : 0.5
σ : 1
E : 2
E : 4
E : 8
Precision
Recall
0.00
0.25
0.50
0.75
1.00
0.0
0.5
1.0

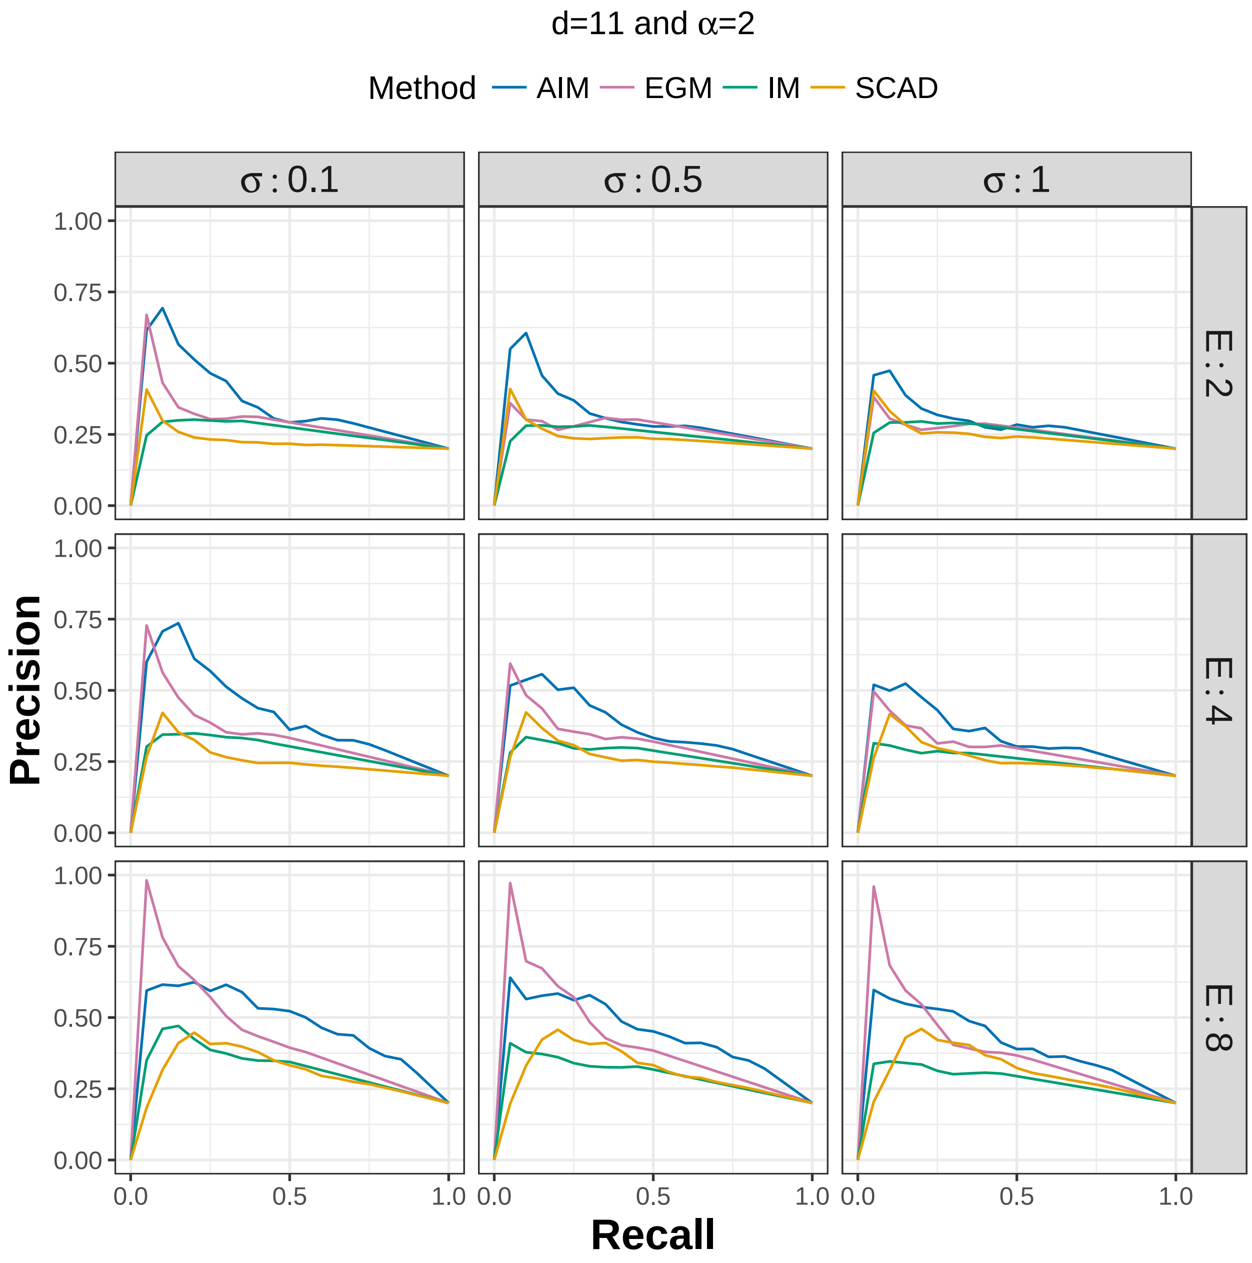

d=11 and α=2
Method AIM EGM IM SCAD
σ : 0.1
σ : 0.5
σ : 1
E : 2
E : 4
E : 8
Precision
Recall
1.00
0.75
0.50
0.25
0.00
0.0
0.5
1.0

Department of Mathematical Sciences, University of Copenhagen, Universitetsparken 5, 2100 Copenhagen Ø, Denmark

*E-mail address*, Corresponding author: `frm@math.ku.dk`

*E-mail address*: `Niels.R.Hansen@math.ku.dk`
